# Supplementary material for: Kalman Filter Auto-tuning through Enforcing Chi-Squared Normalized Error Distributions with Bayesian Optimization
Source: arXiv:2306.07225 source file (2023-06-12)
Supplement: Supplementary file 1 [file appendix.tex]

%appendix.tex
\subsection{Jacobian and Parameters}
\indent The process model for the Skycrane has the form $\dot{\mathbf{x}}(t) = f(\mathbf{x}(t), \mathbf{u}(t)) + \widetilde{\mathbf{w}}$, where
\begin{equation}
    \begin{bmatrix}
        \dot{\xi} \\
        \ddot{\xi} \\
        \dot{z} \\
        \ddot{z} \\
        \dot{\theta} \\
        \ddot{\theta}
    \end{bmatrix}
    = f\left(
    \begin{bmatrix}
        \xi \\
        \dot{\xi} \\
        z \\
        \dot{z} \\
        \theta \\
        \dot{\theta}
    \end{bmatrix}
    ,
    \begin{bmatrix}
        T_1\\
        T_2
    \end{bmatrix}
    \right)
    +
    \begin{bmatrix}
        0 \\
        \widetilde{\omega}_1 \\
        0 \\
        \widetilde{\omega}_2 \\
        0 \\
        \widetilde{\omega}_3 \\
        0
    \end{bmatrix}
\end{equation}
Substituting for Eq.\ \eqref{skycrane_pr_model} and taking derivatives, the Jacobian of the process model is 
\begin{equation}
    \mathbf{F}(t) = 
        \begin{bmatrix}
            0 & 1 & 0 & 0 & 0 & 0 \\
            0 & \mathbf{F}_{11} & 0 & \mathbf{F}_{13} & \mathbf{F}_{14} & 0 \\
            0 & 0 & 0 & 1 & 0 & 0 \\
            0 & \mathbf{F}_{31} & 0 & \mathbf{F}_{33} & \mathbf{F}_{34} & 0 \\
            0 & 0 & 0 & 0 & 0 & 1 \\
            0 & 0 & 0 & 0 & 0 & 0 
        \end{bmatrix}
\end{equation}
where
\begin{equation}\label{J_detail}
    \begin{split}
        \mathbf{F}_{11} &= nc((A_{sc} + A_{bs})(2\dot{\xi}^2 + \dot{z}^2)/V_t + \dot{\xi}\dot{z}(A_{bc} - A_{ss})/V_t ) \\
        \mathbf{F}_{13} &= nc((A_{sc} + A_{bs})(\dot{\xi}+ \dot{z})/V_t + \dot{\xi}^2(A_{ss} - A_{bc})/V_t) \\
        \mathbf{F}_{14} &= l(T_1 \cos{(\beta + \theta)}  + T_2\cos{(\beta-\theta)} + cd \dot{\xi} V_t(A_{ss} - A_{bc}))\\
        \mathbf{F}_{31} &= nc((A_{sc} + A_{bs})(\dot{\xi}+ \dot{z})/V_t) +  \dot{z}^2(A_{bc} - A_{ss})/V_t)\\
        \mathbf{F}_{33} &= nc((A_{sc} + A_{bs})(2\dot{\xi}^2 + \dot{z}^2)/V_t + \dot{\xi}\dot{z}(A_{ss} - A_{bc})/V_t )\\
        \mathbf{F}_{34} &= l(T_2\sin{(\beta-\theta)}-T_1 \sin{(\beta + \theta)} + cd \dot{\xi} V_t(A_{ss} - A_{bc}))
    \end{split}
\end{equation}
Taking derivates of \eqref{skycrane_me_model},
\begin{equation} 
    \begin{split}
        \mathbf{H}(t) = 
            \begin{bmatrix}
                1 & 0 & 0 & 0 & 0 & 0 \\
                0 & 0 & 1 & 0 & 0 & 0 \\
                0 & 0 & 0 & 0 & 0 & 1 \\
                0 & \mathbf{H}_{31} & 0 & \mathbf{H}_{33} & \mathbf{H}_{34} & 0\\
            \end{bmatrix}
    \end{split}
\end{equation}
where
\begin{equation} \label{H_detail}
    \begin{split}
        \mathbf{H}_{31} &= nc((A_{sc} + A_{bs})(2\dot{\xi}^2 + \dot{z}^2)/V_t + \dot{\xi}\dot{z}(A_{bc} - A_{ss})/V_t )\\
        \mathbf{H}_{33} &= nc((A_{sc} + A_{bs})(\dot{\xi}+ \dot{z})/V_t + \dot{\xi}^2(A_{ss} - A_{bc})/V_t)\\
        \mathbf{H}_{34} &= l(T_1 \cos{(\beta + \theta)}  + T_2\cos{(\beta-\theta)} + cd \dot{\xi} V_t(A_{ss} - A_{bc}))
    \end{split}
\end{equation}
The symbols in  \eqref{J_detail} and \eqref{H_detail} are defined as follows
\begin{equation}
    \begin{split}
        cd &= 0.5 \rho C_D \\ 
        l &= \frac{1}{m_f+m_b} \\
        nc &= -0.5 \rho l C_D  \\
        \omega_{cm} &= \frac{\omega_b}{2} \\
        \alpha &= \tan^{-1}(\dot{z}/\dot{\xi}) \\
        V_t    &= \sqrt{\dot{\xi}^2 + \dot{z}^2}\\
        A_s     &= (h_b d_b)+(h_f d_f) \\
        A_b     &= (\omega_b d_b)+(\omega_f d_f)\\
        A_{sc} &= A_s \cos(\theta - \alpha) \\
        A_{ss} &= A_s \sin(\theta - \alpha) \\
        A_{bc} &= A_b \cos(\theta - \alpha) \\
        A_{bs} &= A_b \sin(\theta - \alpha)
    \end{split}
\end{equation}
All the basic constants value are written here
\begin{equation}
    \begin{split}
        \rho &= \SI{0.02}{\kilo\gram\per\metre\cubed}\\
        g &= \SI{3.711}{\meter\per\second\squared} \\
        \beta &= \SI[quotient-mode=fraction]{\pi/4}{\radian} \\
        C_D &= 0.2 \\
        m_f &= \SI{390}{\kilo\gram} \\
        \omega_f &= \SI{1}{\metre} \\
        h_f &= \SI{0.5}{\metre} \\
        d_f &= \SI{1}{\metre} \\
        m_b &= \SI{1510}{\kilo\gram} \\
        \omega_b &= \SI{3.2}{\metre} \\
        h_b &= \SI{2.5}{\metre} \\
        d_b &= \SI{2.9}{\metre} \\
        h_{cm} & = \SI{0.9421}{\metre} \\
    \end{split}
\end{equation}
Mapping between 3 dimensional process noise and 6 dimensional measurement noise $\mathbf{\Gamma}_k$ is 
\begin{equation}
    \mathbf{\Gamma}_k = 
    \begin{bmatrix}
        0 & 0 & 0 \\
        1 & 0 & 0 \\
        0 & 0 & 0 \\
        0 & 1 & 0 \\
        0 & 0 & 0 \\
        0 & 0 & 1 \\
    \end{bmatrix} 
\end{equation}
The fixed measurement noise is 
\begin{equation}
    \widetilde{\mathbf{v}}(t) = (1.0, 0.5, 0.025, 0.0225)^T
\end{equation}
The measurement noise covariance is set as 
\begin{equation}
    \R{k} = 
    \begin{bmatrix}
        1.0 & 0 & 0   & 0\\
        0 & 0.5 & 0   & 0 \\
        0 & 0 & 0.025 & 0 \\
        0 & 0 & 0     & 0.0025 \\
    \end{bmatrix}
\end{equation}

\subsection{Feedback Law of LQR controller}
\indent We need linearize the motion model in order to use LQR controller, e.g. calculating the Jacobian of motion model. We have calculated the Jacobian of motion model with respect to state $\mathbf{x}$. We also need the Jacobian with respect to control $\mathbf{u}$ and noise $\mathbf{w}$ respectively. The Jacobian with respect to control input is 
\begin{equation} \label{jac_control}
    \begin{split}
        \mathbf{U}(t) = 
            \begin{bmatrix}
                0 & 0 \\
                \sin(\theta + \beta)l & \sin(\theta -\beta)l \\
                0 & 0 \\
                \cos(\theta + \beta)l & \cos(\theta - \beta)l\\
                0 & 0 \\
                \frac{1}{I_\eta}(0.5\cos(\beta)\omega_b - \sin(\beta)h_{cm}) & -\mathbf{U}_{50}
            \end{bmatrix}
    \end{split}
\end{equation}
The Jacobian with respect to the noise is
\begin{equation}\label{jac_pnoise}
    \mathbf{W}(t) = 
        \begin{bmatrix}
            0 & 0 & 0 \\
            1 & 0 & 0 \\
            0 & 0 & 0 \\
            0 & 1 & 0 \\
            0 & 0 & 0 \\
            0 & 0 & 1 
        \end{bmatrix}
\end{equation}
Substitute $\x{ref}$ , $\mathbf{u}_{nom}$ into equation \ref{jac_pnoise} and \ref{jac_control} we can get the linearized value of jacobian at the desired point $\mathbf{F}_{\x{ref}}$ and $\mathbf{U}_{\mathbf{u}_{nom}}$. Then the linearized state space model around the desired state can be written as 
\begin{equation}
    \begin{split}
        \dot{\mathbf{x}} &= \mathbf{F}_{\x{ref}} \mathbf{x} +  \mathbf{U}_{\mathbf{u}_{nom}} \mathbf{u} \\
        \mathbf{y} &= \mathbf{x}
    \end{split}
\end{equation}
Then we can get the optimal gain matrix $K_{lin}$ by 
\begin{equation}
    \mathbf{K}_{lin} = \mathbf{R}_{con}^{-1}\mathbf{U}_{\mathbf{u}_{nom}}^T\mathbf{S}_{con}
\end{equation}
where $\mathbf{S}_{con}$ is the solution of of the associated Riccati equation
\begin{equation}
    \begin{split}
        & \mathbf{F}_{\x{ref}}^T \mathbf{S}_{con} + \mathbf{S}_{con}\mathbf{F_{\x{ref}}} - \mathbf{S}_{con}\mathbf{U}_{\mathbf{u}_{nom}}\mathbf{R}_{con}^{-1}\mathbf{U}_{\mathbf{u}_{nom}}^T \\ + & \mathbf{Q}_{con} = \mathbf{0}
    \end{split}
\end{equation}
the $R_{con}$ is a 2 by 2 diagonal matrix with its diagonal element (0.01, 0.01) and the $Q_{con}$ is a 6 by 6 diagonal matrix with its diagonal elements (200 15 200 15 10000 15). Finally we get our $\mathbf{K}_{lin}$
\begin{equation}
    \mathbf{K}_{lin} = 
        \begin{bmatrix}
            100.0 & -100.0 \\
            406.575 & -406.575 \\
            100.0 & 100.0 \\
            519.086 & 519.086 \\
            3053.285 & -3053.285 \\
            3140.470 & -3140.470 \\
        \end{bmatrix}^T
\end{equation}

% you can choose not to have a title for an appendix
% if you want by leaving the argument blank
%\section{}
%Appendix two text goes here.
